# Supplementary material for: The Higher Structure of Symmetries of Axion-Maxwell Theory
Source: arXiv:2411.09685 source file (2025-04-16)
Supplement: Supplementary file 1 [file 3group.tex]

\iffalse
\section{3-groups}\label{Appendix: 3group}
\label{ex: higher group} A $2$-group symmetry is defined by the data $(G^{(0)}, H^{(1)},\rho, \beta)$ of a $0$-form symmetry $G^{(0)}$, a one form symmetry $H^{(1)}$, an action $\rho:\ G^{(0)} \to H^{(1)}$ and $\beta\in H^{3}(G, H)$ describe how the triple fusion $(\eta_{g_1}^{(0)}\otimes \eta_{g_2}^{(0)})\otimes \eta_{g_3}^{(0)}$ sources a defect $\eta_{\beta(g_1,g_2,g_3)}^{(1)}$.

These data reflects in field strengths $H^{(3)}$ for continuous $1$-form symmetries containing nonlinear terms:
\begin{equation}
    H^{(3)}=\dd B^{(2)}-\frac{k}{2\pi}B^{(1)}\dd B^{(1)},
\end{equation}
and unusual gauge transformations:
\begin{equation}
    B^{(1)}\to B^{(1)}+\dd \lambda^{(0)}, \quad B^{(2)}\to B^{(2)}+\dd \lambda^{(1)}+\frac{k}{2\pi}\lambda^{(0)}\dd B^{(1)},
\end{equation}
for the backgrounds $B^{(i)}$.


In fact, recalling that defects correspond to (the Poincaré duals) of flat backgrounds, the non-linear term in the field strengths encodes the information of a Postnikov class $beta$ (in this case $k\in H^{3}(BU(1),U(1))=\Z$), and the gauge transformation both encodes the action $\rho$ end ensures both of these characterizing intersections are topological.

\begin{figure}[ht!]
    \centering\subfloat[Subfigure 1 list of figures text][]{
\includegraphics[width=0.4\textwidth, valign=T]{images/2groups-action between defects.png}\label{fig:action 2group}}
    \subfloat[Subfigure 2 list of figures text][]{
\includegraphics[width=0.5\textwidth,valign=c]{images/2groups-junction2.png} \label{fig:postnikov 2group}}
    \caption{Picturesque representation of the data formin a $2$-group: the action $\rho$ of the $0$-form symmetry on the $1$-form symmetry in \ref{fig:action 2group}, and how a triple intersection of $0$-form symmetry defects sources an $1$-form one in \ref{fig:postnikov 2group} (figures taken from \cite{benini2GroupGlobalSymmetries2019}).}
    \label{fig:Global 2group}
\end{figure}

    
In general, a higher group can be seen as the path groupoid $\mathbf{\Pi}(X)$\footnote{Given a topological space $X$, the objects of the category $\mathbf{\Pi}(X)$ are the points of $X$, morphisms are given by paths, higher morphisms by homotopies and so on.} for a finite homotopy type $X$, i.e. a topological space with a finite number of nontrivial homotopy groups $\pi_i(X)$ each of finite cardinality. Given this setup, the data of a higher group is given higher form symmetries $G^{(i)}=\pi_{i+1}$, by the action of $\pi_1$ on the other homotopy groups and by the $k$-invariants of the Postnikov tower of $X$ (see \cref{AppendixA}). More generally, the structure described in \ref{it: action} is given by the Whitehead product. 
\subsection{Categorical perspective}
\begin{definition}[3 Groups I]
An $n$-group $G^{(n)}$ is a monoidal $(n -1)$-category such that when regarded as a one-object $n$-category $\textbf{B}G^{(n)}$ (via suspension) it becomes a one-object $n$-groupoid, i.e. an $n$-category all whose $k$-morphisms are equivalences, for all $1 \leq k \leq n$.\cite{roberts2008inner}
\end{definition}
\subsection{Algebraic perspective}
\begin{definition}[crossed module]
A pre-crossed module \\ $(H \stackrel{\partial}{\to}G \,, \rhd)$ of groups $G$ and $H$, is given by a group map $\partial : H \to G$,
together with a left action $\rhd$ of $G$ on $H$, by automorphisms, such that for each $h_1\,,h_2 \in H$ and $g \in G$ the following identity hold:
$$g \partial h g^{-1} = \partial (g \rhd h)\,.$$
In a pre-crossed module the {\bf Peiffer commutator} is defined as:
$$
    \left\{ h_1\,,h_2 \right\}=h_1h_2h_1^{-1} \partial(h_1) \rhd h_2^{-1}\,.
$$
A pre-crossed module is said to be a {\bf crossed module} if all of its Peiffer commutators are trivial, which is to say that
$$
(\partial h) \rhd h' = hh'h^{-1}\,,
$$
i.e. the {\bf Peiffer identity} is satisfied.
\end{definition}

\begin{definition}[$2$-crossed module]\fxnote{H,L abelian}
A $2$-crossed module $(L\stackrel{\delta}{\to} H \stackrel{\partial}{\to}G,\,\rhd,\,\{-,\,-\})$ is given by three groups $G$, $H$ and $L$, together with maps $\partial$ and $\delta$ such that:
\begin{displaymath}
    L\stackrel{\delta}{\to} H \stackrel{\partial}{\to}G\,,
\end{displaymath}
where $\partial\delta=1$, an action $\rhd$ of the group $G$ on all three groups, and an $G$-equivariant map called the {\bf Peiffer lifting}:
\begin{displaymath}
\{ - \,,- \} : H\times H \to L\,.
\end{displaymath}
The following identities are satisfied:
\begin{enumerate}
    \item The maps $\partial$ and $\delta$ are $G$-equivariant, i.e. for each $ g \in G$ and $h \in H $:
\begin{equation*}\label{eq:ekvivarijantnost_partial}
    g\rhd \partial (h)=\partial(g\rhd h)\,, \quad \quad \quad g\rhd \delta (l) = \delta(g \rhd l)\,,
\end{equation*}
the action of the group $G$ on the groups $H$ and $L$ is a smooth left action by automorphisms, i.e. for each $g,g_1,g_2 \in G$, $\;h_1,h_2 \in H$, $\;l_1,l_2 \in L$ and $e \in H, L$:
\begin{equation*}\label{eq:ekvivarijantnost_delta}
    g_1 \rhd (g_2 \rhd e) =(g_1 g_2) \rhd e\,, \quad g \rhd (h_1 h_2) =(g \rhd h_1)(g \rhd h_2)\,, \quad g \rhd (l_1 l_2) =(g \rhd l_1)(g \rhd l_2)\,, 
\end{equation*}
and the Peiffer lifting is $G$-equivariant, i.e. for each $h_1,\, h_2 \in H$ and $g \in G$:
$$ g\rhd\{h_1\,,h_2\}=\{ g\rhd h_1, \,g \rhd h_2\}\,;$$
\item the action of the group $G$ on itself is via conjugation, i.e. for each $g\,,g_0 \in G$:
$$ g \rhd g_0 = g\,g_0\,g^{-1}\,;$$
\item In a $2$-crossed module the structure $(L \stackrel{\delta}{\to}H,\,\rhd')$ is a crossed module, with action of the group $H$ on the group $L$ is defined for each $h \in H$ and $l \in L$ as:
$$h \rhd' l = l \, \{\delta(l){}^{-1},\,h\}\,,$$
but $(H \stackrel{\partial}{\to}G \,, \rhd)$ may not be one, and the Peiffer identity does not necessary hold. However, when $\partial$ is chosen to be trivial and group $H$ Abelian, the Peiffer identity is satisfied, i.e. for each $h,\,h' \in H$:
$$\delta(h) \rhd h' = h\, h'\, h^{-1}\,;$$
\item $\delta(\{h_1,h_2 \})= \langle h_1\,,h_2\rangle{}_{\mathrm{p}}$, $\qquad \forall h_1,h_2 \in H$, 
\item $[l_1,l_2]=\{\delta(l_1)\,,\delta(l_2) \}$, $\qquad\forall l_1\,, l_2 \in L$. 
Here, the notation $[l,k]=lkl^{-1}k^{-1}$ is used;
\item $\{h_1h_2,h_3 \}=\{h_1,h_2h_3h_2^{-1} \}\partial(h_1)\rhd \{h_2,h_3 \}$, $\qquad\forall h_1,h_2,h_3 \in H$;

\item $\{h_1,h_2h_3 \}= \{h_1,h_2\} \{h_1,h_3\}\{ \langle h_1,h_3 \rangle{}_{\mathrm{p}}^{-1}, \partial(h_1) \rhd h_2\}$,  {$\qquad\forall h_1,h_2,h_3 \in H$};
\item $\{\delta(l),h\}\{h, \delta(l) \}=l(\partial(h) \rhd l^{-1})$, $\qquad \forall h\in H\,, \quad \forall l \in L$.
\end{enumerate}
\end{definition}
\begin{definition}[$3$-groups II]
Homology of $2$-crossed module    
\end{definition}
\subsection{Topological perspective}
\begin{definition}[$n-$Group III]
    Given a connected topological space $X$ the automorphism of a generic object of the path groupoid $\mathbf{\Pi}X$ is $\infty$-group. If the space is an $n$-type (meaning $\pi_i(X)=0 \ \forall i>n$) the same process give rise to an $n-$group. All $n$-groups actually arise in this manner.
\end{definition}

In this setup, the equivalence classes of the algebraic data above can be nicely interpreted in terms of Postnikov towers.

\begin{definition}[Postnikov]\fxnote{Problemi per $\pi_1$, in particular in that case the data needs an action}
    The idea of a Postnykov system is to build a space one step at a time, increasingly approximating its homotopy type.
    Given a topological space $X$, we denote with $X_{\leq i}$ an $i-$connected space with the same homotopy up to level $i$. 
    The postykov system of a space is given by the data:
    \begin{equation*}
        B^{i+1}\pi_{i+1}\rightarrow X_{\leq i+1} \rightarrow X_{\leq i}
    \end{equation*}
    Each of these sequence is uniquely determined by the $k$-invariant $k\in H^{i+2}(X_{\leq i},\pi_{i+1})=[X_{\leq i},B^{(i+1}\pi_{i+1}]$(we are saying that the fibre of the homotopy pullback is the loop of the target).
    In the general case, one constructs the tower for the universal cover of $X$ and has to find the space in question as:
    \begin{equation*}
        \pi_1\rightarrow\widetilde{X}\rightarrow X
    \end{equation*}
    i.e. action of $\pi_1$ on $\widetilde{X}$
\end{definition}
In this setup, the Piffer commutator, for example, is hidden in the $k$-class in $H^4(B^2\pi_2,\pi_3)$. This group is in fact given by the group of quadratic forms, and the $k$-class of a specific space is a quadratic refinement of the withead product (in the case of trivial fundamental group).

\begin{definition}[Withehead product]
Bilinear maps:
\begin{equation*}
    [\bullet,\bullet]: \pi_i(X)\times \pi_j(X)\rightarrow \pi_{i+j-1}(X)
\end{equation*}
    Given by following the diagram
    \begin{equation*}
        \begin{aligned} S^{ n_1 + n_2 -1 } & \overset{ f_{n_1,n_2} }{ \longrightarrow } & S^{n_1} \vee S^{n_2} & \overset{ (\phi_1, \phi_2) }{\longrightarrow} & X \\ \big\downarrow &  & \big\downarrow \\ D^{ n_1 + n_2 } &\underset{}{\longrightarrow}& S^{n_1} \times S^{n_2} \end{aligned}
    \end{equation*}
    related to the skeletal decomposition of $D^{i+j}$, where it is always useful to imagine things as hyper-squares
\end{definition}
\begin{remark}
    There is somehow an action of $\pi_1$ on the other homotopy groups, I don't know if it is related to whitehed product
\end{remark}
\subsection{Physical perspective}
\fi
